# Supplementary material for: Subspace Hybrid MVDR Beamforming for Augmented Hearing
Source: arXiv:2311.18689 source file (2023-11-30)
Supplement: Supplementary file 1 [file appendices.tex]

% if have a single appendix:
%\appendix[Proof of the Zonklar Equations]
% or
%\appendix  % for no appendix heading
% do not use \section anymore after \appendix, only \section*
% is possibly needed

% use appendices with more than one appendix
% then use \section to start each appendix
% you must declare a \section before using any
% \subsection or using \label (\appendices by itself
% starts a section numbered zero.)
%
\appendices
\input{minimisation_proof}
\label{sec:minimisation}

% you can choose not to have a title for an appendix
% if you want by leaving the argument blank
% \section{}
% % \input{appendix_two}
% Appendix two text goes here.
% \appendix
% \label{appendix:minimisation_proof}
% \input{minimisation_proof}
